# Supplementary material for: Power-Scalable Generation of High-Order Optical Vortices Via Coherent Beam Combining
Source: arXiv:2512.19815 ancillary file (2025-12-25)
Supplement: Supplementary file 1 [file supplementary.pdf]

# Supplementary information for :

# Power-Scalable Generation of High-Order Optical Vortices Via Coherent Beam Combining

**Hossein Fathi[1,*], Rafael F. Barros[2], and Regina Gumenyuk[1]**

[1]Laboratory of Photonics, Physics Unit, Faculty of Engineering and Natural Sciences, Tampere University, Korkeakoulunkatu 3, 33720 Tampere, Finland
[2]Instituto de Física, Universidade de São Paulo, 05315-970 São Paulo, SP, Brazil
[*]hossein.fathi@tuni.fi

## Coherent beam combining of Gaussian beams

This section presents the results of coherent beam combining (CBC) of Gaussian beams, which serve as a reference for comparison with the CBC results of optical vortices (OVs).

### Beam quality, polarization, and combining efficiency assessment of Gaussian beams

Fig. S1 illustrates the assessment of beam quality, degree of polarization (DOP), and combining efficiency for Gaussian beams. Fig. S1a shows the near-field beam profiles of the individual channels and the coherently combined beam, along with their measired beam quality $M^2$ factors. The average DOP for both the individual channels and the coherently combined Gaussian beams was measured using 2,000 consecutive readings taken with a commercial polarimeter (PAX1000IR2/M, Thorlabs). A maximum combining efficiency of 96.2% was achieved at 100 W average output power, serving as a benchmark for comparison with the CBC performance of OVs. The 3.8% combining loss is primarily attributed to spatial amisalignment, as well as beam asymmetry and size mismatch among the individual beams. Combining efficiency is defined as the ratio of the output power of the combined beam to the total output power of all individual input laser beams prior to combining.

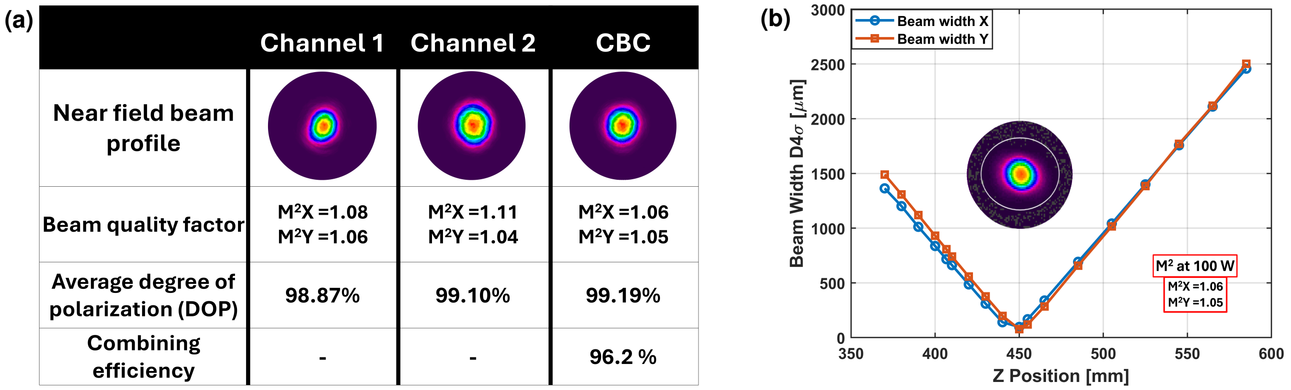


**Figure 1.** Beam quality, polarization, and combining efficiency assessment of Gaussian beams. (a) Near-field beam profiles of two individual linearly polarized Gaussian beams and their coherently combined output, accompanied by the corresponding degree of polarization and measured combining efficiency. (b) $M^2$ curve of the coherently combined Gaussian beam, recorded at 100 W average output power. Insets show the beam profile of the combined Gaussian beam at the focus plane of the lens of the $M^2$ measurement system.

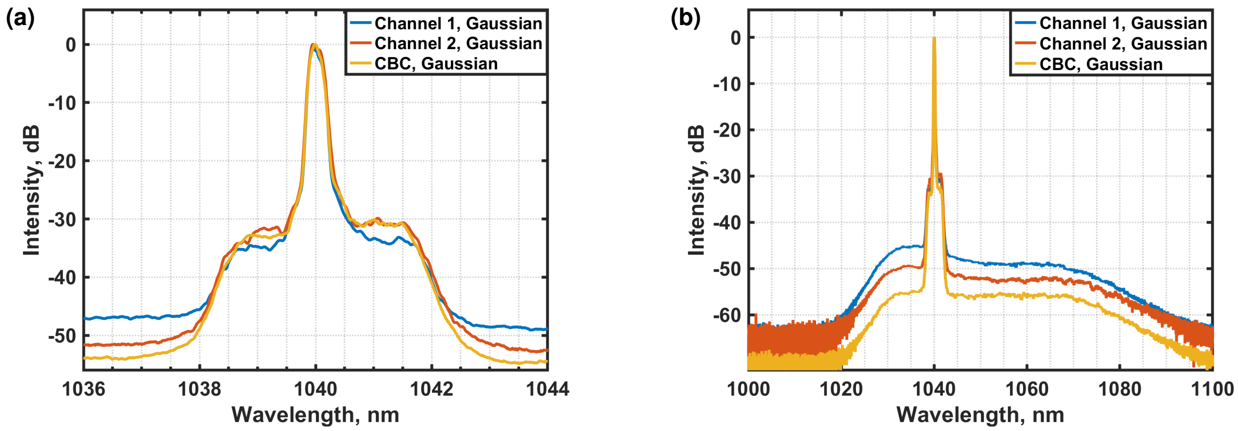


**Figure 2.** Optical spectrum characterization of the individual channels and the combined Gaussian beam. (a), (b); Output optical spectra of both individual channels and the coherently combined Gaussian beam within the narrow and wide spectral range, respectively.

---

The beam profiles of the individual channels measured at 55 W exhibit slight asymmetries, as reflected in the corresponding $M^2$ values along the $x$- and $y$-axes (see Fig. S1a). In contrast, the combined beam measured at 100 W shows a substantially more uniform intensity distribution. This improvement in beam quality, relative to the individual channels, is attributed to coherent filtering effects[1]. Fig.S1b presents the $M^2$ curve of the coherently combined Gaussian beam, with insets showing the corresponding beam profile at the focal plane of the lens in the $M^2$ measurement system.

### Optical spectrum assessment of the CBC of Gaussian beams

Fig. S2 shows representative optical spectra of the individual channels and the coherently combined Gaussian beam over both narrow and wide spectral ranges. Fig. S2a displays the spectra within a narrow bandwidth for the individual beams (measured at an average output power of 55 W) and the combined beam (measured at 100 W). The broader spectral characteristics are depicted in Fig. S2b. The combined beam exhibits a higher signal-to-amplified spontaneous emission (ASE) ratio, indicating the effect of coherent filtering. The spectral shoulders observed in the individual beams, primarily arising from ASE, are incoherent in both phase and polarization and are thus not present in the combined output.

## Coherent beam combining of Optical vortices

This section presents the results of coherent beam combining of the optical vortices.

### Beam quality assessment of OVs

There is not a single standardized parameter (like the beam quality factor for Gaussian beams) for quantifying OVs. The quality of OVs is often described by several parameters, such as intensity distribution profile and mode purity. Fig.S3 presents the beam quality assessment of the coherently combined OVs using the ISO 11146-compliant $M^2$ method, which characterizes the focusing ability of the beams relative to an ideal Gaussian beam. The $M^2$ curves for combined beams with topological charges $\ell = 1$, 5, and 8 are shown, with inset displaying the beam profile of the OV with $\ell = 8$ at the focal plane of the measurement system, as a representative case. The theoretical beam quality values for ideal, aberration-free OVs are provided in Eq. 1 for reference.

$$M^2 = 2p + |\ell| + 1 \tag{1}$$

where $\ell$ represents the topological charge and $p$ denotes the radial mode[2].

### Mode content assessment of OVs

A detailed mode decomposition analysis was performed on both the individual channels and the coherently combined beams for OVs with topological charges $\ell = 1$, 5, and 8. The mode decomposition for a given complex field distribution $U(r)$ is calculated as

$$P_\ell = \frac{|\mathscr{O}_\ell|^2}{\sum_m |\mathscr{O}_m|}, \quad \mathscr{O}_m = \int d^2r\, U(r) \exp(-im\phi), \tag{2}$$

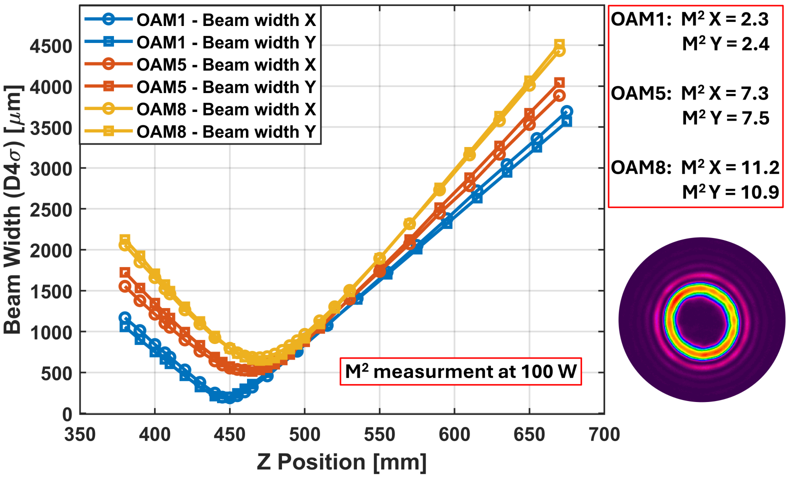


**Figure 3.** Beam quality assessment of CBC of Optical vortices at 100 W. $M^2$-curve of the combined beams of OVs with $\ell = 1$, 5, and 8 (Inset: The beam profile of the combined OAM with $\ell = 8$ at the focus plane of the lens of the $M^2$ measurement system).

---

where $\mathscr{O}_m$ represents the inner product of the complex field with a spiral phase of topological charge $m$. Importantly, the mode content $\{P_\ell\}$ depends strongly on the alignment between the measured field and the simulated spiral phase. To ensure an accurate estimation of the modal content, we implement spatial and angular offsets in the measured field distribution to maximize the overlap of each optical vortex with its target mode. The spatial shifts are implemented simply by shifting the acquired images laterally, while for the angular offsets, we add a constant phase gradient to the complex field. The magnitudes of the offsets are optimized using a standard genetic algorithm implemented in MATLAB.

As illustrated in Fig. 4, panels (a–c) show the modal content for the two individual beams and their combined output with $\ell = 1$. Similarly, panels (d–f) and (g–i) present the corresponding analyses for $\ell = 5$ and $\ell = 8$, respectively. The decomposition quantifies the percentage contributions of various orbital angular momentum (OAM) components within each beam, enabling a precise evaluation of mode purity. The combined optical vortices consistently exhibit superior modal properties compared to the average of the individual beams, highlighting the coherent filtering effect intrinsic to the CBC technique[1], independent of the topological charge of the OVs. This analysis reveals how effectively the coherent beam combining preserves the dominant mode while minimizing unwanted OAM components, thereby confirming the high quality and mode purity of the combined output.

## References


1. Brignon, A. *Coherent Laser Beam Combining*. ISBN:978-3-527-41150-4 (John Wiley & Sons, 2013).
2. Mabena, C. M., Bell, T., Mphuthi, N., Harrison, J. & Naidoo, D. Beam quality factor of aberrated Laguerre-Gaussian optical beams. *Opt. Express* **31**, 26435–26450, DOI: 10.1364/OE.493594 (2023).

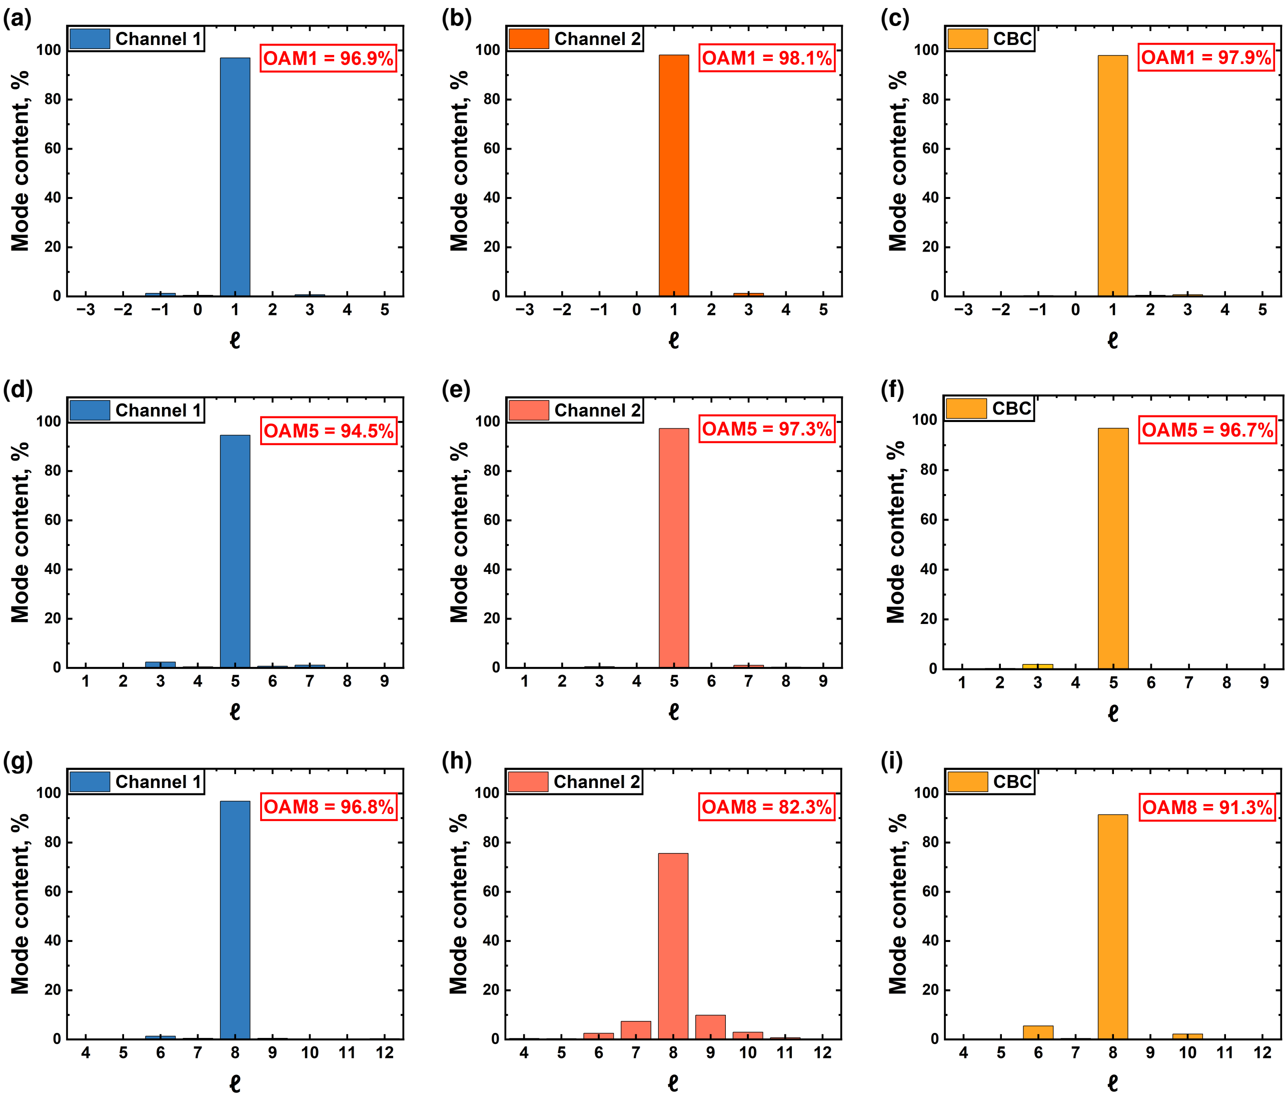


**Figure 4.** Mode decomposition analysis of the individual and coherently combined beams for OVs with topological charges $\ell = 1$, 5, and 8. (a–c) Mode content of the two individual channels and the combined output for $\ell = 1$. (d–f) Same analysis for $\ell = 5$. (g–i) Same analysis for $\ell = 8$. In each case, the decomposition shows the percentage contributions of different OAM components, indicating the purity of the main mode.
